# Supplementary material for: Realizable Continuous-Space Shields for Safe Reinforcement Learning
Source: arXiv:2410.02038 source file (2024-12-02)
Supplement: Supplementary file 1 [file liveness-extended.tex]

\subsection{Encoding Non-Markovian Requirements}
\label{sec:app:liveness-requirements}

LTLt, \cite{rodriguez2023boolean} is a specification language expressive enoough to reason about both time and data.
Moreover, using precise specifications of dynamics that the domain holds (essentially, Thm.~\ref{th:method:decidable}), in Ex.~\ref{ex:nonMarkovian} we showed that we can also enconde non-markovian properties that contain data.

\begin{example} \label{ex:properties}
    The following is a simplified encoding of the queues used in Sec.~\ref{sec:caseStudy}.
    
    Consider the only parameter to check is that a visited region $\text{reg} \in R$ in the arena is not visited for the next $k$ timesteps, then, we encode this property as follows: for all $\text{reg} \in R$, it holds that $\square [(x,y) \in \text{reg} \rightarrow \diamond_{[1,k]} (x,y) \notin \text{reg}]$, provided that the system cannot play to avoid that $(x,y) \in \text{reg}$ eventually happens (i.e., for all $\text{reg} \in R$, it also holds that $\diamond (x,y) \in \text{reg}$.
     
\end{example}

However, certification of such realizability (or unrealizability) is difficult to interpret for the designers, because it captures an explosion of combination of environment and system dynamics.

\begin{example}
    We attach in the supplementary zip a \texttt{dotfiles.org} with several graphs in \texttt{dotgraph} format to represent the strategies of the shields as automata\footnote{We also show the encoding in LTLt, the realizability result and the abstraction for Strix \cite{meyer18explicit}, which is the tool we used for realizability checking. Note that we are using Boolean abstractions as suggested by \cite{rodriguez2023boolean}. }. 
    These show how very simple non-markovian specifications like the ones in Ex.~\ref{ex:properties} very quickly become not easy to explain.
    \texttt{Shield(1,1)} encodes a single (temporaly) forbidden region with a single timestep horizon.
   \texttt{Shield(2,1)} encodes a single forbidden region with a two timestep horizon.   
   \texttt{Shield(3,1)} encodes a single forbidden region with a three timestep horizon.
    We can see it that this size only increases linearly.
    However, we have to add another dimension: more (temporaly) forbidden regions.
    \texttt{Shield(1,2)} encodes a single (temporaly) forbidden region with a single timestep horizon.
    \texttt{Shield(2,3)} encodes a single (temporaly) forbidden region with a two timestep horizon.
    Note that this interpretation complexity grows exponentially (see figures for \texttt{Shield(1,1)}, \texttt{Shield(1,2)} and \texttt{Shield(2,2)} at the end of the appendices), but also note that realizability checking procedure's running time remains in seconds.
\end{example}

This suggests that like real-life non-markovian LTLt properties need to be defined encoded different way.
Therefore, in this paper we propose
shields that model non-markovian specifications, but all of them encoded as markovian specifications for the safety properties \textbf{plus} a stateful (thus, finite) memory that we called \textit{history} $H$ in Sec.~\ref{sec:method}. Since $H$ is stateful, decidability of this method is not compromised.
It is very important to note that $H$ has to hold certain properties depending on the domain of the problem:
\begin{itemize}
    \item Certain elements $h \in H$ cannot be followed by other $h'$. For instance, if the robot is region $x \in [0,10], y \in [0,10]$ in $h$ of position $i$, it cannot be in $x \in [800,900], y \in [800,900]$ in $h'$ of position $i+1$.
    \item The last $h$ in $H$ represents exactly the combination of the constraints that the previous state 
    $(x,y,r)$ satisfied and the constraints that previous movement $(a^0,a^1)$ satisfied. It is easy to see that the amount of combinations here is finite.
    \item It is not possible that, given arbitrary $h, h' \in H$, $h=h'$, which means that elements in $H$ cannot be repeated.
    \item Entries are related throughout time: i.e., if $h \in H$ appears in position $i$ in timestep $k$, it will be in position $i-1$ in timestep $k+1$.
\end{itemize}
Note again that these properties rely completely in the domain of the problem.

Then, if we guarantee these assumptions of the environment, we can specify the properties of the system in a straightforward manner: in every timestep, hold safety properties (inherently markovian) plus do not allow the output $o$ to be such that $o\in h$, for every $h \in H$.
This way, we can build a lightweight\footnote{In the sense that it will have way less states and thus will be easier to interpret.} shield that conform to the guarantees, whereas we delegate the assumptions to some other checker (which can be a synthetised model of the environment or any other \textbf{verified} program).
This yields extremely simple shields with more or less states that depend on the safety specifications and not the combinations of the non-markovian specifications.

In general, we can formally express this in the LTL synthesis notation as follows:

\begin{theorem}
\label{th:method:nonMarkov}

If a non-markovian specification $\varphi$ is realizable using stateful memory as an environment variable, then the property $\varphi'$ that encoding such memory as bounded-liveness in the side of the system is also realizable.
\end{theorem}

\begin{proof}
    
The proof sketch goes as follows: $\varphi$ is an over-approximation of the power of the environment in which we allow it to choose freely the values for $H$ in each timestep, and then we weaken this freedom by the properties like the aforementioned ones (e.g., no repeated element). Since $\varphi$ is an over-approximation of the power of the environment and it is realizable, then the version $\varphi'$
in which this power is not over-approximated is also necessarily realizable.

\end{proof}

\subsection{Figures of Shields} \label{subsec:figures}

We show below the strategies computed from three non-markovian specifications of Ex.~\ref{ex:nonMarkovian}.
The idea is to see how quickly they get difficult to interpret.

\begin{figure}[]
\centering
\includegraphics[width=0.3\linewidth]{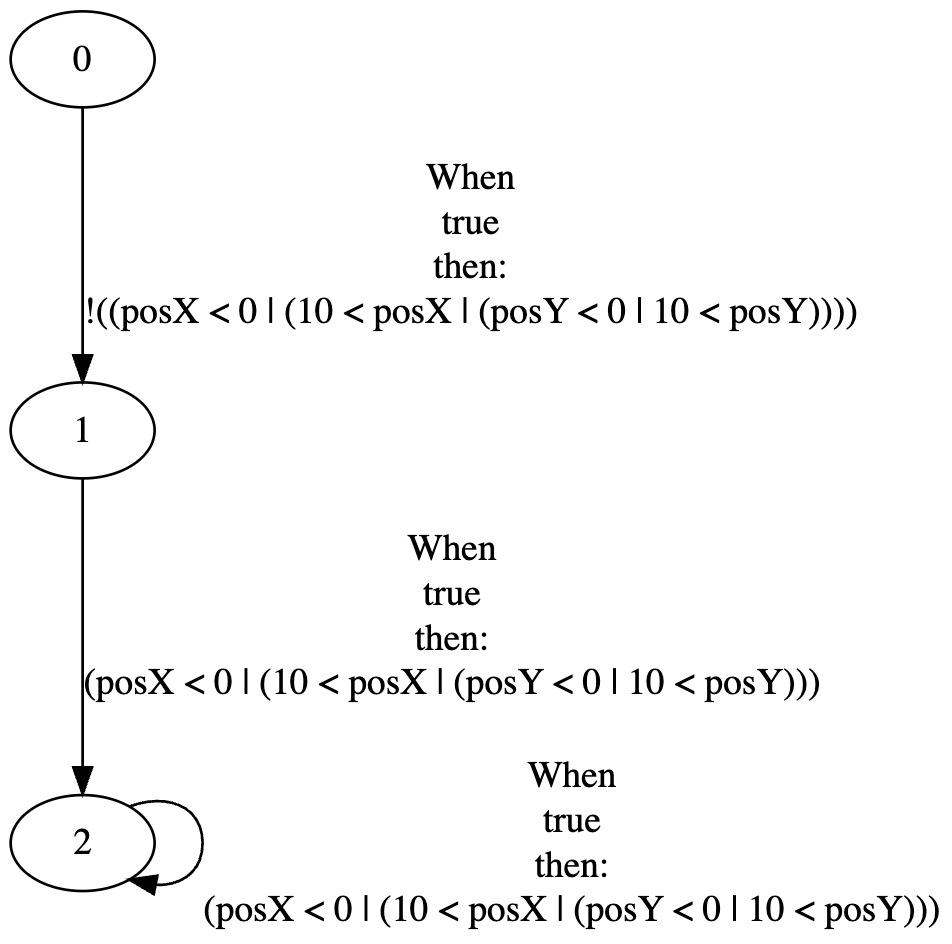} 
% \minipage{0.48\linewidth}
%     \includegraphics[width=\linewidth]{example-image-a} 
% \endminipage \hfill
% \minipage{0.48\linewidth}
%     \includegraphics[width=\linewidth]{example-image-b} 
% \endminipage
\caption{\texttt{Shield(1,1)}.}

\end{figure}

\begin{figure}[]
\centering
\includegraphics[width=1.0\linewidth]{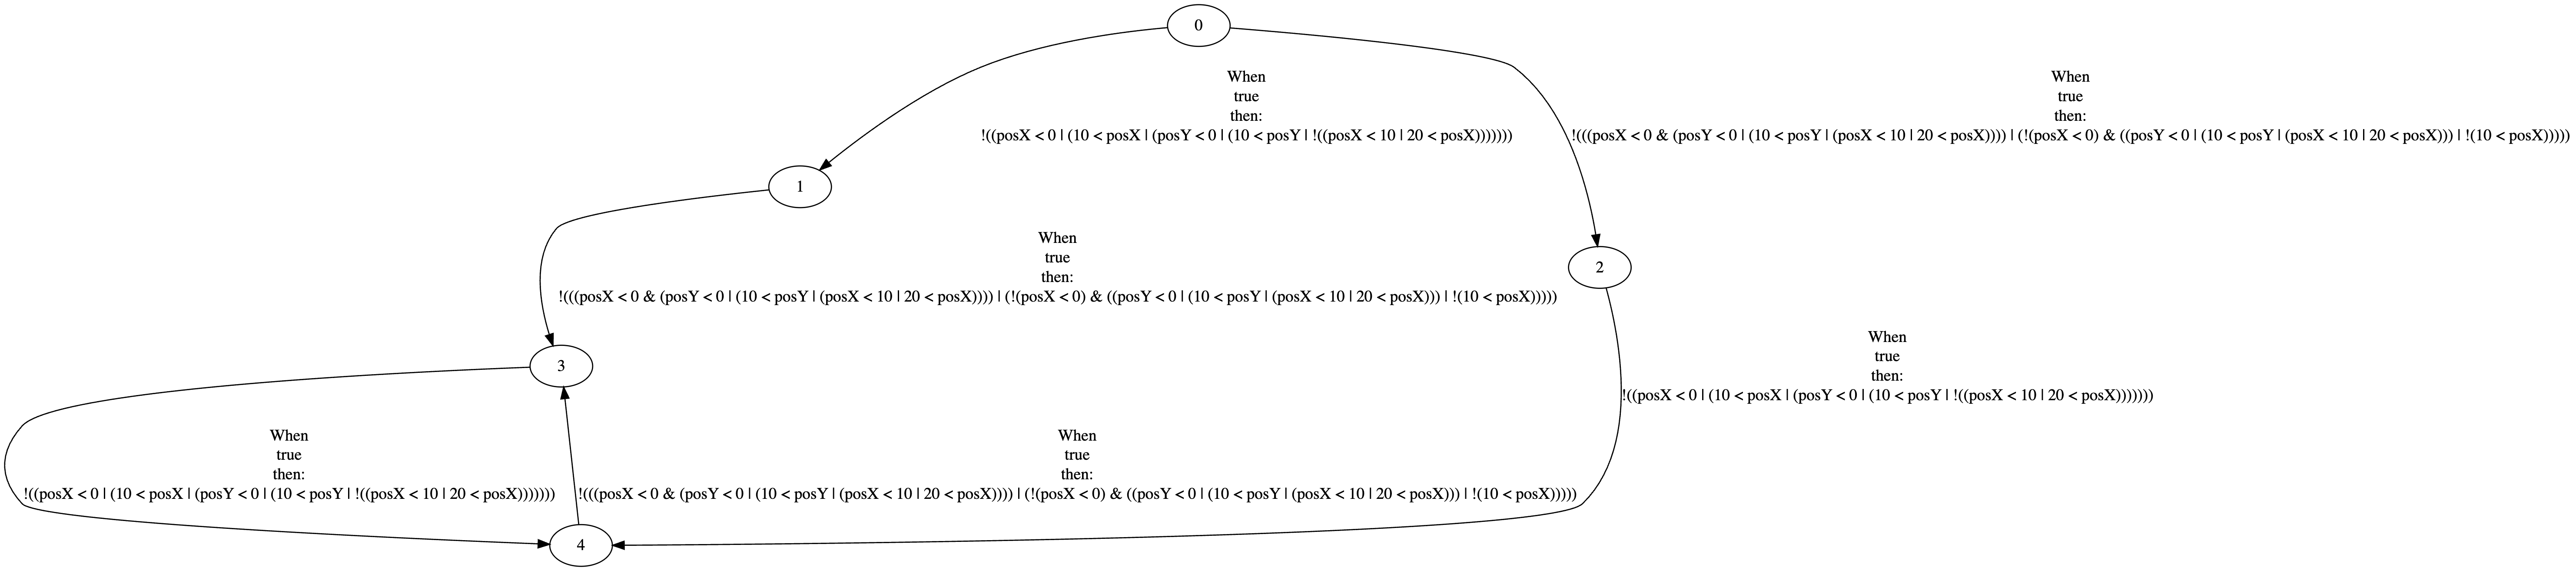} 
% \minipage{0.48\linewidth}
%     \includegraphics[width=\linewidth]{example-image-a} 
% \endminipage \hfill
% \minipage{0.48\linewidth}
%     \includegraphics[width=\linewidth]{example-image-b} 
% \endminipage
\caption{\texttt{Shield(1,2)}.}

\end{figure}

\begin{figure}[]
\centering
\includegraphics[width=1.0\linewidth]{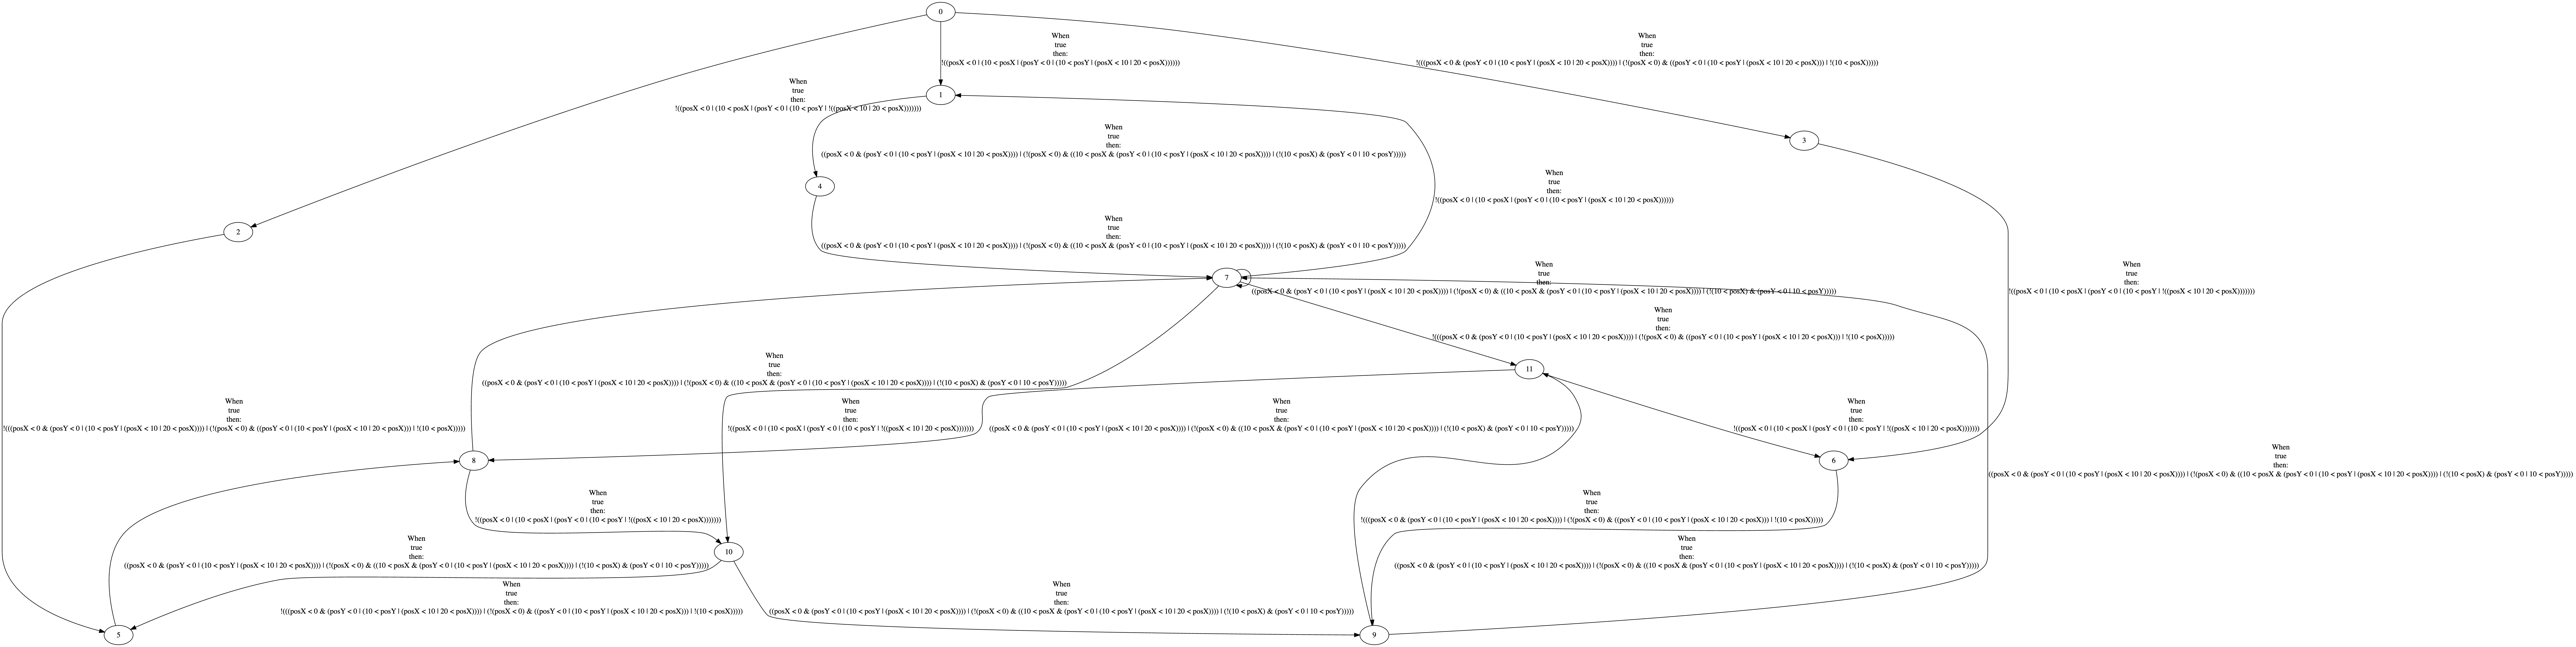} 
% \minipage{0.48\linewidth}
%     \includegraphics[width=\linewidth]{example-image-a} 
% \endminipage \hfill
% \minipage{0.48\linewidth}
%     \includegraphics[width=\linewidth]{example-image-b} 
% \endminipage
\caption{\texttt{Shield(2,2)}.}

\end{figure}
