# Supplementary material for: Realizable Continuous-Space Shields for Safe Reinforcement Learning
Source: arXiv:2410.02038 source file (2024-12-02)
Supplement: Supplementary file 2 [file reproducibility.tex]

\section*{Reproducibility Checklist}

This paper
\begin{itemize}
\item Includes a conceptual outline and/or pseudocode description of AI methods introduced (\textbf{yes})
\item Clearly delineates statements that are opinions, hypotheses, and speculations from objective facts and results (\textbf{yes})
\item Provides well-marked pedagogical references for less-familiar readers to gain the background necessary to replicate the paper (\textbf{yes})
\end{itemize}

Does this paper make theoretical contributions? (\textbf{yes})
If yes, please complete the list below.

\begin{itemize}
\item All assumptions and restrictions are stated clearly and formally. (\textbf{yes})
\item All novel claims are stated formally (e.g., in theorem statements). (\textbf{yes})
\item Proofs of all novel claims are included. (\textbf{yes})
\item Proof sketches or intuitions are given for complex and/or novel results. (\textbf{yes})
\item Appropriate citations to theoretical tools used are given. (\textbf{yes})
\item All theoretical claims are demonstrated empirically to hold. (\textbf{yes})
\item All experimental code used to eliminate or disprove claims are included. (\textbf{no})
\end{itemize} 

Does this paper rely on one or more datasets? (\textbf{no}) \\

Does this paper include computational experiments? (\textbf{yes})
If yes, please complete the list below.

\begin{itemize}
\item Any code required for pre-processing data is included in the appendix. (\textbf{no})
\item All source code required for conducting and analyzing the experiments is included in a code appendix. (\textbf{partial})
\item All source code required for conducting and analyzing the experiments will be made publicly available upon publication of the paper with a license that allows free usage for research purposes. (\textbf{yes})
\item All source code implementing new methods have comments detailing the implementation, with references to the paper where each step comes from (\textbf{partial})
\item If an algorithm depends on randomness, then the method used for setting seeds is described in a way sufficient to allow replication of results. (\textbf{partial})
\item This paper specifies the computing infrastructure used for running experiments (hardware and software), including GPU/CPU models; amount of memory; operating system; names, and versions of relevant software libraries and frameworks. (\textbf{yes})
\item This paper formally describes the evaluation metrics used and explains the motivation for choosing these metrics. (\textbf{yes})
\item This paper states the number of algorithm runs used to compute each reported result. (\textbf{yes})
\item Analysis of experiments goes beyond single-dimensional summaries of performance (e.g., average; median) to include measures of variation, confidence, or other distributional information. (\textbf{yes})
\item The significance of any improvement or decrease in performance is judged using appropriate statistical tests (e.g., Wilcoxon signed rank). (\textbf{partial})
\item This paper lists all final (hyper-)parameters used for each model/algorithm in the paper’s experiments. (\textbf{partial})
\item This paper states the number and range of values tried per (hyper-) parameter during the development of the paper, along with the criterion used for selecting the final parameter setting. (\textbf{partial})
\end{itemize}
