# Supplementary material for: Realizable Continuous-Space Shields for Safe Reinforcement Learning
Source: arXiv:2410.02038 source file (2024-12-02)
Supplement: Supplementary file 3 [file safety-extended.tex]

\section{LTLt Details}

Since, due to space limitations, we could not formally explain two intuitions on how to use LTL modulo theories of \cite{rodriguez2023boolean} for our solution, we now detail them. In addition, the formal encoding of the requirements is available in the supplementary material; \textit{dotfiles.org} contains the specification in LTL, while the Python encoding is available in \textit{shield.py}.

\subsection{Relating Timesteps}
\label{sec:app:safety-requirements}

An essential observation used for this paper is that, using continuous domains with no uncertainty, we can usually \textit{anticipate} the dangerous movement of the system, because each valuation of $(a^0, a^1)$ in state $(x,y,r)$ induces a very precise next state.
This allows us to specify all the desired properties in decidable fragments of LTLt.

We capture this intuition more formally as follows: 

\begin{theorem}
\label{th:method:decidable}
Given a variable $v$ in $\varphi$, if the following conditions hold:
\begin{itemize}
    \item Valuation of $v$ in a future timestep $k_{\text{future}}$ can be fully inferred from a valuation in a previous step $k_{\text{past}} < k_{\text{future}}$; 
    \item and $v$ in $k_{\text{past}}$ only relates to variables in $k_{\text{past}}$ and $v$ in $k_{\text{future}}$ only relates to variables in $k_{\text{future}}$
\end{itemize}

Then every property expressed using $\lhd$ can also be expressed in an non-cross-state (NCS) formula.
\end{theorem}

\begin{proof}

The proof sketch goes as follows: Given the conditions on $v$ presented in the theorem, we can rewrite any formula containing $\lhd v$; concretely, 
$\lhd v$ can be replaced with a formula $\psi(v_{k_{\text{past}}})$ that only depends on the valuation of $v$ and other variables in the previous timestep $k_{\text{past}}$.
This is possible because the valuation of $v$ in the future timestep $k_{\text{future}}$ can be fully determined from the valuation in the previous timestep $k_{\text{past}}$.
By applying this rewriting, any formula containing $\lhd v$ can be transformed into an NCS formula that does not cross state boundaries. This is because the future state information is fully captured in the formula $\psi(v_{k_{\text{past}}})$, which only depends on the previous state.
    
\end{proof}
